# Supplementary material for: Generalization of Quasi-Newton Methods: Application to Robust Symmetric Multisecant Updates
Source: arXiv:2011.03358 source file (2021-02-08)
Supplement: Supplementary file 1 [file convergence_quadratic.tex]

\section{Convergence Analysis for Quadratics}\label{QuadraticProof}

\subsection{Convergence analysis for minimizing quadratic functions}

In this section we analyse the convergence rate of quasi-Newton methods when $f$ is the quadratic function
\[
	f(x) = \frac{1}{2}(x-x^*)^TQ(x-x^*), \quad Q \succ 0.
\]
For such function, the gradient is written
\[
	\nabla f(x) = Q(x-x^*).
\]
In this case, there is a strong link between the matrices $\DX$ and $\DG$ since
\begin{equation}
	\DX = Q\DG, \qquad \Leftrightarrow Q^{-1}\DX = \DG.
\end{equation}

In this section, we consider any method of the form
\begin{equation}
	x_{k+1} = x_k-H_k\nabla f(x_k) \label{eq:qnstep}
\end{equation}
where $H_k$ satisfies \textit{exactly} the secants conditions
\[
	H_k \DG = \DX.
\]
We show that this family of method has the optimal rate of convergence
\[
	\| \nabla f(x_k) \|_M = \min_{p\in\Pone{k}} \| p(Q) \nabla f(x_0) \|_M,
\]
where $\Pone{k}$ is the set of polynomials with degree at most $k$ whose coefficients sum to one, and
\[
	\| v \|_M = \sqrt{ v^T M v}, \quad M\succ 0.
\]

The next proposition shows the structure of the matrix $H_k$, if it satifies the secant conditions.
\begin{proposition} \label{prop:formula_h}
	If the function is quadratic, the matrix $H_k$ is written
	\[
		H_k = \DX(\DG)^\dagger + \tilde H(I-\DG(\DG)^\dagger)
	\]
	where $(\DG)^\dagger$ is a pseudo inverse of $\DG$ satisfying
	\[
		\DG(\DG)^\dagger\DG = \DG.
	\]
\end{proposition}
\begin{proof}
	Since $H_k$ satisfies the secant conditions, $H_k$ can be written as
	\[
	H_k = \DX(\DG)^\dagger
	\]
	where $(\DG)^\dagger$ is a pseudo inverse of $\DG$ satisfying
	\[
	\DG(\DG)^\dagger\DG = \DG.
	\]
	In this case, it satisfies the secant conditions since $(I-\DG(\DG)^\dagger)\DG = 0$ and
	\[
		H_k \DG = \DX(\DG)^\dagger\DG = Q^{-1}\DG(\DG)^\dagger\DG = Q^{-1}\DG = \DX.
	\]
\end{proof}

\subsection{Generalized qN step}
We introduce the generalized qN step, written
\begin{equation}
	x_{k+1} = (X - H_k G) c \label{eq:generalized_qnstep}
\end{equation}
where $c$ is a vector whose entries sum to one, and
\[
	X = [x_0, \, \ldots, \, x_k], \quad G = [\nabla f(x_0), \, \ldots, \, \nabla f(x_k)].
\]
The qN update \eqref{eq:qnstep} can be seen as a special case of \eqref{eq:generalized_qnstep} where $c = [0,\,\ldots,\, 0,\, 1]^T$. The nest proposition shows that for any $c$, the step \eqref{eq:generalized_qnstep} is identical.
\begin{proposition}\label{prop:invariant_c}
	For any $c,\,c'$, the generalized qN step \eqref{eq:generalized_qnstep} produce the same $x_k$, i.e.,
	\[
		(X - H_k G) (c-c') = 0. 
	\]
\end{proposition}
\begin{proof}
	With proposition \ref{prop:formula_h}, we have
	\[
		H_k = \DX(\DG)^\dagger.
	\]
	Thus, the difference between two generalized qN step  is written 
	\[
		(X - \DX(\DG)^\dagger G +  \tilde H(I-\DG(\DG)^\dagger) G) (c-c'). 
	\]
	Since $c$ and $c'$ sum to one, $(c-c')$ sum to zero. Consider the $k\times k-1$ matrix 
	\[
		C =\begin{bmatrix}
		1 \\
		-1 & 1 \\
		0 & -1 & 1\\
		& & \ddots & \ddots
		\end{bmatrix}.
	\]
	Then, it is easy to show that $C$ is full column rank and 
	\[
		\DX = XC, \qquad \DG = GC.
	\]
	In addition, for any vector $w$ with $k-1$ entries that sum to zero, there exists a vector $v$ such that
	\[
		w = Cv.
	\]
	In particular, we consider the vector $v$ that gives
	\[
		Cv = (c-c').
	\]
	We thus have
	\[
		\tilde H(I-\DG(\DG)^\dagger) G (c-c') = \tilde H(I-\DG(\DG)^\dagger) \DG v = 0
	\]
	and
	\begin{eqnarray*}
		(X - \DX(\DG)^\dagger G) (c-c')  & = & (X - \DX(\DG)^\dagger G) Cv, \\
		& = & (\DX - \DX(\DG)^\dagger \DG)v,\\
		& = & Q^{-1}(\DG - \DG(\DG)^\dagger \DG)v\\
		& = & Q^{-1}(\DG - \DG)v,\\
		& = & 0.
	\end{eqnarray*}
\end{proof}

\subsection{Accuracy of the generalized qN step}

In this section, we consider the generalized qN step, where $\DG$ and $\DX$ are full column rank. At the end of this section we will consider the case where $\DG$ and $\DX$ are not full rank. The next proposition gives the expression of the gradient of the generalized $qN$ step.
\begin{proposition}\label{prop:formula_gradient}
	The gradient of $x_{k+1}$, generated by the generalized qN iteration \eqref{eq:generalized_qnstep} is written
	\[
		\nabla f(x_{k+1}) = (I-Q\tilde H)(I-P)Gc \qquad \forall c:c^T1=1.
	\]
	where $P = \DG(\DG)\dagger$.
\end{proposition}
\begin{proof}
	The gradient of $x_{k+1}$ is written
	\[
		\nabla f(x_{k+1}) = Q(x_{k+1}-x^*) = Q((X - H_k G)c - x^*) \qquad \forall c:c^T\textbf{1} = 1,
	\]
	which is valid for all $c$ that sum to one thanks to Proposition \ref{prop:invariant_c}. If we writte
	\[
		X^* = [x^* x^* \ldots] = x^*\textbf{1}^T,
	\]
	then, because $\textbf{1}^Tc = 1$ we have
	\[
		Q(x_{k+1}-x^*) = Q((X - H_k G)c - x^*) = Q(x_{k+1}-x^*) = Q((X-X^* - H_k G)c).
	\]
	In addition, it is easy to show that $Q(X-X^*) = G$. Thus,
	\[
		Q(X-X^* - H_k G)c =  (G - QH_k G)c.
	\]
	Finally, using the definition of $H_k$ from Proposition \eqref{prop:formula_h},
	\begin{eqnarray*}
		\nabla f(x_{k+1}) & = & (G - Q\DX(\DG)^\dagger G + Q\tilde H(I-\DG(\DG)^\dagger) G)c,\\
		& = & (I - \DG(\DG)^\dagger - Q\tilde H(I-\DG(\DG)^\dagger) ) Gc.
	\end{eqnarray*}
	Writting $P = \DG(\DG)^\dagger $, we finally have
	\[
		\nabla f(x_{k+1}) =  (I - P - Q\tilde H(I-P ) Gc = (I-Q\tilde H)(I-P)Gc.
	\]
\end{proof}
Intuitively, this means the gradient of the point $x_{k+1}$ is equal to zero in the space generated by $P$, and in its orthogonal space the better $\tilde H$ approximates $Q^{-1}$, the smaller the norm of the gradient is.

Before going further, we need to prove the following lemma.

\begin{lemma} \label{lem:wtf_lemma}
	There exist a $c^*$ such that $\textbf{1}^T(c^*) = 1$ and
	\[
		(I-P)Gc^* = Gc^*.
	\]
	Moreover, if $G_{k+1} = [G, \, \nabla f(x_{k+1})]$ is also full rank then the last coefficient $c^*_{k+1}$ is nonzero.
\end{lemma}
\begin{proof}
	If we want $(I-P)Gc^* = Gc^*$, it is sufficient to find $c^*$ such that
	\[
		PGc^* = 0, \qquad \Leftrightarrow \quad c \in \ker(PG) .
	\]
	However, the matrix $PG$ of size $k\times k+1$ can be at most of rank $k$. Thus, the dimension of its kernel it at least one. Now, we will show by contradiction that, if the vector $c^*$ sum to 0, then it cannot be a non-trivial solution of the system. 
	
	Indeed, if $c^T\textbf{1} = 0$ then there exists a vector $v$ such that $Gc = \DG v$ (see proof of Proposition \ref{prop:invariant_c}). In this case,
	\[
		PGc^* = P\DG v = \DG(\DG)^\dagger\DG v = \DG v = Gc^*.
	\]
	However, because the matrix $G$ is full column rank, it is impossible to find a non-zero $c^*$ such that $Gc^* = 0$.
	
	In conclusion, there exists a solution $c^*$ such that $c^*\in\ker(PG)$ and $\textbf{1}^Tc^* = 1$. 
	
	Now, we need to show that its last coefficient is nonzero if $\nabla f(x_{k+1})$ is linearly independant of previous gradients, i.e., 
	\[
		\rank( [G, \nabla f(x_{k+1})] )= k+2 \quad \Rightarrow \quad c^*_{k+1} \neq 0.
	\]
	We now use the optimal $c^*$ to write the gradient $\nabla f(x_{k+1})$. Indeed, combined with Proposition \ref{prop:formula_gradient}, we have
	\[
		\nabla f(x_{k+1}) = (I-Q\tilde H)Gc^*.
	\]
	Writing $c^{(i)}$ the optimal vector obtained for the gradient $\nabla f(x_i)$, we have
	\[
		G_{1\ldots k+1} = [\nabla f(x_{1}), \ldots, \nabla f(x_{k+1})] =  (I-Q\tilde H)G\begin{bmatrix}
			c^{(1)} & c^{(2)} & \ldots & c^{(k)} & c^{(k+1)} \\
			0_{k\times 1} & 0_{(k-1)\times 1} & \ldots & 0_{1\times 1} & 
		\end{bmatrix}.
	\]
	Clearly, the matrix of $c$'s is upper-triangular. Thus, if $[G, \nabla f(x_{k+1})]$ is full rank, $G_{1\ldots k+1}$ is also full rank. Thus, it is necessary to the matrix of $c$'s to have non-zero elements in the diagonnal, so $c_{k+1}^{(k+1)}=c_{k+1}^*\neq 0$.
\end{proof}

With this lemma we can now show that qN can be seen as Krylov methods, under some conditions on the matrix $\tilde H$.

\begin{proposition}\label{prop:grad_polynomial}
	Assume $G$ full column rank. Then, $\nabla f(x_k)$ can be written
	\[
		\nabla f(x_{k+1}) = p_{k+1}(I-Q\tilde H)\nabla f(x_0)
	\]
	where $p_{k+1}$ is a polynomial of degree $k+1$ (i.e. its leading coefficient is nonzero) and its coefficients sum to one $(i.e. p(1) = 1)$.
\end{proposition}
\begin{proof}
	Using Lemma \ref{lem:wtf_lemma} and Proposition \ref{prop:formula_gradient}, the gradient can be written
	\[
	\nabla f(x_{k+1}) = (I-Q\tilde H)Gc^{*}
	\]
	for some $c$ such that $\textbf{1}^Tc^* = 1$ and $c^*_{k+1}\neq 0$ (i.e, it sums to one and the last coefficient is nonzero). We show by recursion that
	\[
	\nabla f(x_{k+1}) = p_{k+1}(I-Q\tilde H)\nabla f(x_0)
	\]
	where $p_{k+1} \in \Pone{k+1}$, the set of polynomial whose coefficients sum to one with nonzero leading coefficients. Of couse, the first element satisfies this condition since
	\[
	\nabla f(x_0) = (I-Q\tilde H)^0 \nabla f(x_0) = p_0(I-Q\tilde H)\nabla f(x_0),
	\] 
	for the particular polynomial $p_0(z) = 1$. Now assume this is true for all $\nabla f(x_i)$ up to $i=k$. In this case,
	\begin{eqnarray*}
		\nabla f(x_{k+1}) & = & (I-Q\tilde H)Gc^{*}\\
		& = &(I-Q\tilde H)\sum_{i=1}^{k+1} c_i^* \nabla f(x_{i-1})\\
		& = & \underbrace{(I-Q\tilde H)\sum_{i=1}^{k+1} c_i^* p_{i-1}(I-Q\tilde H)}_{=p_{k+1}(I-Q\tilde H)}\nabla f(x_0)
	\end{eqnarray*}
	Clearly, $p_{k+1}(I-Q\tilde H)$ is a polynonial of degree at most $k+1$ since it corresponds to a linear combination of polynomials of degree at most $k$, then multiplied by $(I-Q\tilde H)$. It is easy to see that the coefficients of $p_{k+1}$ sum to one, since
	\[
	p_{k+1}(1) = (1)\sum_{i=1}^{k+1} c_i^* p_{i-1}(1)
	\]
	By recurtion, all $p_{i-1}(1) = 1$ and by assumption $\textbf{1}^Tc^*_i = 1$. Now we need to show that the leading coefficient is nonzero. The highest degree polynomial is the following,
	\[
	c_{k+1}^* (I-Q\tilde H)p_{k}(I-Q\tilde H)
	\] 
	By recursion, the degree of $p_k$ is \textit{exactly} $k$, thus its leading coefficient is nonzero. Moreover, it comes with a non-zero contribution since $c_{k+1}^*$ is non-zero by Lemma \eqref{lem:wtf_lemma}. This means that $p_{k+1}$ has degree \textit{exactly} $k+1$.
\end{proof}

This proposition shows us that we are iteratively building a basis of polynomials. This is a crucial point in our proof, as now we are abble to show that the rate of convergence of multisecants qN method is similar to the rate of conjugate gradients or GMRES.

\begin{theorem} \label{thm:rate_convergence}
	If we use a multisecant qN method, then for all $M \succ 0$,
	\begin{equation}
		\| \nabla f(x_k)\|_M \leq \|I- M^{1/2}Q\tilde HM^{-1/2}\| \min_{p\in\Pone{k}} \|p(I-Q\tilde H) \nabla f(x_0) \|_M \label{eq:rate_convergence_general}
	\end{equation}
\end{theorem}
\begin{proof}
	We start with the result of Proposition \ref{prop:formula_gradient},
	\[
		\nabla f(x_{k+1}) = (I-Q\tilde H)(I-P)Gc \qquad \forall c:c^T1=1.
	\]
	First, we consider the projector
	\[
		(I-\tilde P) = (I-Q\tilde H)(I-P)(I-Q\tilde H)^{-1}.
	\]
	Since the formula is valid \textit{for all $c$} that sum to one, we can pick $c$ such that
	\[
		c^{opt} = \argmin{c:c^T\textbf{1} = 1} \|(I-Q\tilde H)(I-P)Gc \|_M
	\]
	for a positive definite matrix $M$. In this case,
	\begin{eqnarray}
	    & & \|\nabla f(x_{k+1})\|_M \\
	    & = & \|(I-Q\tilde H(I-P)Gc^{opt}\|_M\\
		& = & \min_{c:\textbf{1}^Tc=1}\|(I-Q\tilde H)(I-P)Gc\|_M\\
		& \leq & \|M^{1/2}(I-Q\tilde H)M^{-1/2}\|_2 \|M^{1/2}(I-P)M^{-1/2}\|_2 \min_{c:\textbf{1}^Tc=1} \|Gc\|_M
	\end{eqnarray}
	We have that $M^{1/2}(I-P)M^{-1/2}$ is also a projector, thus its norm is bounded by one. By consequence,
	\[
		 \|\nabla f(x_{k+1})\|_M \leq \|M^{1/2}(I-Q\tilde H)M^{-1/2}\|_2 \min_{c:\textbf{1}^Tc=1}\|Gc\|_M
	\]
	By Proposition \ref{prop:grad_polynomial}, we have that the $i-th$ column of $G$ represent a polynomial of degree \textit{exactly} $i-1$, whose coefficients sum to one. Thus, by combining the $k+1$ columns of $G$ with coefficients $c$ that also sum to one, we can build any polynomial of $\Pone{k}$. This means
	\[
		\min_{c:\textbf{1}^Tc=1} \|(I-Q\tilde H)Gc\|_M = \min_{p\in \Pone{k}} \|(I-Q\tilde H)p(I-Q\tilde H)\nabla f(x_0)\|_M
	\]
	This prove the desired result.
\end{proof}

In the particular case where $0 \preceq I-Q\tilde H \preceq 1-\kappa$ and $M=I$, we can show a rate similar to conjugate gradients method.

\begin{corollary} \label{cor::convergence_minimal_polynomial}
	Let $\zeta$ the degree of the minimal polynomial of $(I-Q\tilde H)$, and assume $Q\tilde H$ invertible. If $(I-Q\tilde H)$ is symmetric, $0 \preceq I-Q\tilde H \preceq 1-\kappa \prec I$ and $M=I$, 
	\[
		\|\nabla f(x_{k+1})\|_2 \leq \begin{cases}
			2(1-\kappa) \left(\frac{1-\sqrt{\kappa}}{1+\sqrt{\kappa}}\right)^k \|\nabla f(x_{k+1})\|_2 & \text{if } k\leq \zeta \\
			0  & \text{if } k > \zeta
		\end{cases}
	\]
\end{corollary}
\begin{proof}
	It suffices to split de norm in Theorem \ref{thm:rate_convergence} as follow,
	\[
		\|\nabla f(x_{k+1})\|_2 \leq  \underbrace{\|I-Q\tilde H\|_2}_{\leq 1-\kappa} \|\nabla f(x_0) \|_2 \min_{p\in\Pone{k}} \| p(I-Q\tilde H) \|_2
	\]
	Then, using classical results for minimal polynomial (see for instance~\citep{golub2012matrix}), we have that, if $k\leq \zeta $,
	\[
		\min_{p\in\Pone{k}} \| p(I-Q\tilde H) \|_2 \leq \min_{p\in\Pone{k}} \max_{A: 0\preceq A \preceq 1-\kappa} \| p(A) \|_2 \leq 2\left(\frac{1-\sqrt{\kappa}}{1+\sqrt{\kappa}}\right)^k.
	\]
	Otherwise, consider $q$ the minimal polynomial of $I-Q \tilde H$. Since $Q \tilde H$ is invertible, the matrix $I-Q \tilde H$ does not have $1$ as eigenvalue, thus $q(1) \neq 0$. In this case, $p = \frac{q}{q(1)}$ is a feasible solution of \eqref{eq:rate_convergence_general}, so
	\[
		\min_{p\in\Pone{k}} \|p(I-Q\tilde H) \nabla f(x_0) \|_M \leq \|q(I-Q\tilde H) \nabla f(x_0) \|_M = 0
	\]
	by definition of the minimal polynomial.
\end{proof}

\newpage
